# Supplementary material for: Topics in Effective Field Theory for Lattice QCD
Source: arXiv:hep-lat/0608010 source file (2006-08-16)
Supplement: Supplementary file 1 [file BMassAppendix.tex]

\chapter{\label{app:BaryonMasses} Baryon Mass Appendices}

%%%%%%%%%%%%%%%%%%%%%%%%%%%%%%%%%%%%%%%%%%%%%%%%%%%
%
%	SU(3) masses
%
%%%%%%%%%%%%%%%%%%%%%%%%%%%%%%%%%%%%%%%%%%%%%%%%%%%
 \section{Baryon Masses in $SU(3)$ HB$\chi$PT \label{app:SU3masses}}

%%%%%%%%%%%%%%%%%%%%%%%%%%%%%%%%%%%%%%%%%%%%%%%%%%%
%
%	Gell-Mann Okubo violation to m_q^2
%
%%%%%%%%%%%%%%%%%%%%%%%%%%%%%%%%%%%%%%%%%%%%%%%%%%%
\subsection*{\textbf{Deviation of the Gell-Mann--Okubo mass relation through $\mc{O}(m_q^2)$}}

As an application, we would just like to note that the octet baryon mass expressions can be used to compute the expected deviations of the Gell-Mann--Okubo mass relation of the octet baryons~\cite{Okubo:1961jc,Ne'eman:1961cd,Gell-Mann:1962xb}.  However, a recent lattice QCD computation has found that the deviations of this relation are small for a range of pion masses which are only as light as $m_\pi \sim 294$~MeV~\cite{Beane:2006pt}.  Thus, any signal for the $\mc{O}(m_q^2)$ corrections will likely be dominated by the $\mc{O}(m_q^{3/2})$ corrections, which were used in Ref.~~\cite{Beane:2006pt}.

%%%%%%%%%%%%%%%%%%%%%%%%%%%%%%%%%%%%%%%%%%%%%%%%%%%
%
%	SU(6|3) masses
%
%%%%%%%%%%%%%%%%%%%%%%%%%%%%%%%%%%%%%%%%%%%%%%%%%%%
 \section{Baryon Masses in $SU(6|3)$ HB$\chi$PT \label{app:PQSU63masses}}
